# Supplementary material for: Wasserstein Distances, Geodesics and Barycenters of Merge Trees
Source: arXiv:2107.07789 source file (2021-09-20)
Supplement: Supplementary file 1 [file appendixRest.tex]

% \section{Minimizing the Fr\'echet energy}

% \section{$\distanceSequence(\mathcal{S}, \mathcal{S}')$ is a metric}

\newpage
\section{Draft -- Fr\'echet energy and geodesics}
\label{sec_draft}
As in \cite{Turner2014} we use the Fr\'echet energy as the function to optimize 
in order to find the barycenter of a set. In their work they use persistence 
diagrams, here we use merge trees, especially, their branch decomposition. In 
the following we use the term merge tree to represent their branch 
decomposition.

We define the Wasserstein barycenter 
$\branchtree^*$ of a set 
$\branchtreeSet = \{\branchtree(f_1), \dots, \branchtree(f_N)\}$ of merge trees 
as the minimizer of the Fr\'echet energy of the set, under our metric 
$\wassersteinTree$. It is the merge tree $\branchtree^* \in \branchtreeSpace$ (where 
$\branchtreeSpace$ is the space of merge trees and where $\alpha_i$ are 
coefficients that sums up to 1 and such that $\forall i \; \alpha_i \in [0, 1]$) that 
minimizes its \emph{average} distance to the merge trees of the set:

\begin{eqnarray}
 \branchtree^* = 
    \argmin_{\branchtree \in \branchtreeSpace}
      \sum_{\branchtree(f_i) \in \branchtreeSet}
        \alpha_i
        \wassersteinTree\big(\branchtree, \branchtree(f_i)\big)^2
\end{eqnarray}

\subsection{Special case with 2 trees}

At first, we have focused on the simplest special case where the number of trees in the set is 2. Moreover, it will permits us to define geodesics between two merge trees. In this special case, the Fr\'echet energy can be defined as:

\begin{eqnarray}
 F(\alpha) = 
        \alpha
        \wassersteinTree\big(\branchtree, \branchtree(f_1)\big)^2
        + (1-\alpha)
        \wassersteinTree\big(\branchtree, \branchtree(f_2)\big)^2
\end{eqnarray}

Where $\branchtree$ is the interpolated branch decomposition merge tree with nodes interpolated from the ones in the first one $\branchtree(f_1)$ to the ones in the second tree $\branchtree(f_2)$. We show that this tree actually minimizes the Fr\'echet energy.

The goal here is to compute the partial derivatives of the Fr\'echet energy according the parameters we want to estimate and find solutions of these equations. The parameters are the scalar values of each node (corresponding to the birth and death of a persistence pair) in $\branchtree$. 

Let $\phi : \branchtree(f_1) \to \branchtree(f_2)$ be an optimal pairing between nodes of $\branchtree(f_1)$ and nodes of $\branchtree(f_2)$. We want to construct $\branchtree$ with nodes being linearly interpolated from $\branchtree(f_1)$ to $\branchtree(f_2)$ according $\phi$. This means that we construct $\phi' : \branchtree(f_1) \to \branchtree$ and $\phi'' : \branchtree \to \branchtree(f_2)$ such that $\phi'(i) = z$ and $\phi''(z) = j$ if $\phi(i) = j$. Using this construction we have in $\wassersteinTree\big(\branchtree, \branchtree(f_1)\big)^2$ a cost $\gamma(i \to z)$ and in $\wassersteinTree\big(\branchtree, \branchtree(f_2)\big)^2$ a cost $\gamma(z \to j)$.
We show that this strategy effectively minimizes the Fr\'echet energy.

Since a node can only be matched/inserted/deleted once, each cost in the Fr\'echet energy involves independent nodes in $\branchtree$. When computing the partial derivatives according the parameters of a node, it will remains in the equation only the derivative of the cost related to this node, all other costs being treated as constant and therefore removed of the equation. It means that each matching/insertion/deletion can be treated independently

\paragraph{\textbf{Matching case.}}

Let a node $i$ in the $\branchtree(f_1)$, a node $j$ in the $\branchtree(f_2)$ and $\phi(i) = j$ we want to estimate the parameters of a node $z$ in $\branchtree$ that goes from $i$ to $j$. The parameters associated to the node $z$ are the scalar values $z_b$ and $z_d$ of the persistence pair to which it corresponds. We can then compute the partial derivatives of the Fr\'echet energy according the parameters to estimate. 

We recall the cost of matching $i$ to $z$ and $z$ to $j$:

\begin{align}
\begin{split}
\gamma(i \to z) = &\left(\cfrac{i_b - \delta_{min}}{\delta_{max} - \delta_{min}} - \cfrac{z_b - \mu_{min}}{\mu_{max} - \mu_{min}}\right)^2\\
+ &\left(\cfrac{i_d - \delta_{min}}{\delta_{max} - \delta_{min}} - \cfrac{z_d - \mu_{min}}{\mu_{max} - \mu_{min}}\right)^2
\end{split}
\end{align}

\begin{align}
\begin{split}
\gamma(z \to j) = &\left(\cfrac{z_b - \mu_{min}}{\mu_{max} - \mu_{min}} - \cfrac{j_b - \eta_{min}}{\eta_{max} - \eta_{min}}\right)^2\\ 
+ &\left(\cfrac{z_d - \mu_{min}}{\mu_{max} - \mu_{min}} - \cfrac{j_d - \eta_{min}}{\eta_{max} - \eta_{min}}\right)^2
\end{split}
\end{align}

These costs are included in $\wassersteinTree\big(\branchtree, \branchtree(f_1)\big)^2$ and $\wassersteinTree\big(\branchtree, \branchtree(f_2)\big)^2$ respectively. We can then compute the partial derivatives of $F(\alpha)$ given $z_b$ and $z_d$:

\begin{align}
    \frac{\partial F(\alpha)}{\partial z_b} = \cfrac{2 \bigg(\alpha \cfrac{i_b-\delta_{min}}{\delta_{min} - \delta_{max}} + (1-\alpha)\cfrac{j_b-\eta_{min}}{\eta_{min} - \eta_{max}} + \cfrac{z_b - \mu_{min}}{\mu_{max} - \mu_{min}}\bigg)}{\mu_{max} - \mu_{min}}
\end{align}

\begin{align}
    \frac{\partial F(\alpha)}{\partial z_d} &= \cfrac{2 \bigg(\alpha \cfrac{i_d-\delta_{min}}{\delta_{min} - \delta_{max}} + (1-\alpha)\cfrac{j_d-\eta_{min}}{\eta_{min} - \eta_{max}} + \cfrac{z_d - \mu_{min}}{\mu_{max} - \mu_{min}}\bigg)}{\mu_{max} - \mu_{min}}
\end{align}

By solving these equations we can found the following solutions:

\begin{align}
\begin{split}
    z_b &= \left(\alpha \cfrac{i_b-\delta_{min}}{\delta_{max} - \delta_{min}} + (1-\alpha)\cfrac{j_b-\eta_{min}}{\eta_{max} - \eta_{min}}\right) (\mu_{max} - \mu_{min}) + \mu_{min} \\
\end{split}   
\end{align}

\begin{align}
\begin{split}
    z_d &= \left(\alpha \cfrac{i_d-\delta_{min}}{\delta_{max} - \delta_{min}} + (1-\alpha)\cfrac{j_d-\eta_{min}}{\eta_{max} - \eta_{min}}\right) (\mu_{max} - \mu_{min}) + \mu_{min} \\
\end{split}   
\end{align}

We can notice that these solutions are a generalized case of the classical interpolation $\alpha x + (1-\alpha) y$ where we introduce normalization terms.

We now show that the scalar values associated to the node $z$ are always in the interval of the ones of its parent. This allows to verify that the interpolated merge tree has a valid structure. We show this in the following for the birth value $z_b$ but everyting holds in the same way of the death value $z_d$.

We know by definition that $i_b \in [\delta_{min}, \delta_{max}]$ and $j_b \in [\eta_{min}, \eta_{max}]$ therefore $\frac{i_b-\delta_{min}}{\delta_{max} - \delta_{min}}, \frac{j_b-\eta_{min}}{\eta_{max} - \eta_{min}} \in [0, 1]$.

The interpolated value $\alpha x + (1-\alpha) y$ of two reals $x, y \in [0, 1]$ is in the interval $[0, 1]$. It means that $\alpha \frac{i_b-\delta_{min}}{\delta_{max} - \delta_{min}} + (1-\alpha)\frac{j_b-\eta_{min}}{\eta_{max} - \eta_{min}} \in [0, 1]$. We then multiply this value by $(\mu_{max} - \mu_{min})$, the interval then become $[0, (\mu_{max}-\mu_{min})]$, finally we add $\mu_{min}$ meaning that the result is in $[\mu_{min}, \mu_{max}]$.

\paragraph{\textbf{Deletion/Insertion case.}}

In this case we consider a node $i$ in $\branchtree(f_1)$ such that $\phi(i) = \Delta(i)$ (with $\Delta(i) = \frac{i_b+i_d}{2}$, the projection on the diagonal in the birth/death space). The insertion case, where we consider a node $j$ in $\branchtree(f_2)$ such that $\phi(\Delta(j)) = j$ is symmetric. We want to estimate the parameters $z_b$ and $z_d$ of a node $z$ in $\branchtree$ that goes from $i$ to $\Delta(i)$ (or $\Delta(j)$ to $j$ in the insertion case).

\begin{align}
\begin{split}
    \frac{\partial F(\alpha)}{\partial z_b} = &-2 \alpha \left(\cfrac{i_b - \delta_{min}}{\delta_{max} - \delta_{min}} - \cfrac{z_b - \mu_{min}}{\mu_{max} - \mu_{min}}\right) / (\mu_{max} - \mu_{min}) \\ 
    &+ (1 - \alpha) \cfrac{z_b - z_d}{(\mu_{max} - \mu_{min})^2} 
\end{split}   
\end{align}

\begin{align}
\begin{split}
    \frac{\partial F(\alpha)}{\partial z_d} = &-2 \alpha \left(\cfrac{i_d - \delta_{min}}{\delta_{max} - \delta_{min}} - \cfrac{z_d - \mu_{min}}{\mu_{max} - \mu_{min}}\right) / (\mu_{max} - \mu_{min}) \\
    &- (1 - \alpha) \cfrac{z_b - z_d}{(\mu_{max} - \mu_{min})^2}
\end{split}   
\end{align}

To treat this case we need to solve a system with the two equations above since $z_b$ appears in the partial derivative of $z_d$ and vice versa. By doing so we can actually found solutions very similar to the matching case:

\begin{align}
\begin{split}
    z_b &= \left(\alpha \cfrac{i_b-\delta_{min}}{\delta_{max} - \delta_{min}} + (1-\alpha)\cfrac{ \Delta(i) -\delta_{min}}{\delta_{max} - \delta_{min}}\right) (\mu_{max} - \mu_{min}) + \mu_{min} \\
\end{split}   
\end{align}

\begin{align}
\begin{split}
    z_d &= \left(\alpha \cfrac{i_d-\delta_{min}}{\delta_{max} - \delta_{min}} + (1-\alpha)\cfrac{ \Delta(i) -\delta_{min}}{\delta_{max} - \delta_{min}}\right) (\mu_{max} - \mu_{min}) + \mu_{min} \\
\end{split}   
\end{align}

Once again we know that the final result will be in $[\mu_{min}, \mu_{max}]$ for the same reason than the matching case.

\subsection{General case with $n$ trees}

\begin{align}
\begin{split}
    \frac{\partial F(\alpha)}{\partial z_b} &= - 2 \left(-\cfrac{z_b - \mu_{min}}{\mu_{max} - \mu_{min}} + \sum_i \alpha_i \cfrac{\phi_i(z)_b-\delta_{min}^i}{\delta_{max}^i - \delta_{min}^i}\right) / (\mu_{max} - \mu_{min}) 
\end{split}   
\end{align}
    
\begin{align}
\begin{split}
    \frac{\partial F(\alpha)}{\partial z_d} &= - 2 \left(-\cfrac{z_d - \mu_{min}}{\mu_{max} - \mu_{min}} + \sum_i \alpha_i \cfrac{\phi_i(z)_d-\delta_{min}^i}{\delta_{max}^i - \delta_{min}^i}\right) / (\mu_{max} - \mu_{min}) 
\end{split}   
\end{align}

\begin{align}
\begin{split}
    z_b &= \left( \sum_i \alpha_i \cfrac{\phi_i(z)_b-\delta_{min}^i}{\delta_{max}^i - \delta_{min}^i} \right) (\mu_{max} - \mu_{min}) + \mu_{min} \\
\end{split}   
\end{align}

\begin{align}
\begin{split}
    z_d &= \left( \sum_i \alpha_i \cfrac{\phi_i(z)_d-\delta_{min}^i}{\delta_{max}^i - \delta_{min}^i} \right) (\mu_{max} - \mu_{min}) + \mu_{min} \\
\end{split}   
\end{align}
